# Supplementary material for: Cheetah: Optimizing and Accelerating Homomorphic Encryption for Private Inference
Source: arXiv:2006.00505 source file (2020-10-08)
Supplement: Supplementary file 1 [file 11-appendix.tex]

% \begin{figure}[t]
% \centering
% \subfloat[CNN]{\includegraphics[width=0.45\textwidth]{figures/cnn_val.pdf}}\\
% \vspace{-1em}
% \subfloat[FC]{\includegraphics[width=0.45\textwidth]{figures/fc_val_format.pdf}}
% %\hspace{1em}
% \vspace{-1em}
% \caption{
% Performance and noise models validation.
% Axis labels starting with 0, 1, and 2, are tested with HE parameters:
% ($n$, $t$, $q$, $w_{pt}$, $w_{ct}$) = (2048, 19, 60, 19, 22), 
%  (2048, 19, 60, 10, 16),
%  (4096, 18, 60, 18, 24), respectively
% (unit is in bits except $n$).
% CNN parameters: ($w, f_w, c_i, c_o$), FC parameters: ($n_i, n_o$)
% %\fixme{Describe fc and cnn params.} \YI{ legend for black dash?}
% }
% \label{app:model_val}
% \end{figure}

% \appendix
% \section{Appendix}
% \subsection{Benchmarks}\label{app:benchmarks}

% Cheetah is evaluated using six deep learning models spanning different scales
% from MNIST~\cite{lecun1998gradient},
% to CIFAR-10~\cite{krizhevsky2009learning}
% and ImageNet~\cite{russakovsky2015imagenet}.
% For MNIST, LeNet5 and LeNet-300-100 models are used~\cite{lecun1998gradient}.
% CIFAR-10 models are AlexNet~\cite{krizhevsky2012imagenet} and 
% an 8-layer CNN with 7-CONV and 1-FC used in \cite{liu2017oblivious}.
% Finally for ImageNet, 
% VGG16~\cite{simonyan2014very}, 
% and ResNet50~\cite{he2016deep} are used.
%Note that while some of these benchmarks may seem small,
%this is the first paper on HE for DL that considers ResNet50.
